# Supplementary material for: DyadMem: A Long-Term Memory Benchmark of How Agents Work with Users
Source: arXiv:2610.03020 source file (2026-10-02)
Supplement: Supplementary file 1 [file Ethics_statement.tex]

This work does not involve human subjects or the collection of private user data. The benchmark dataset is constructed from synthetic user--agent interactions. We acknowledge that LLM-generated data may contain biases or artifacts; therefore, we employ automated checks, human review, and sampling-based quality checks to ensure data quality. This benchmark is intended solely for research purposes and may not fully represent the diversity of real-world users.
